# Supplementary material for: One-Shot Transfer of Affordance Regions? AffCorrs!
Source: arXiv:2209.07147 source file (2022-09-16)
Supplement: Supplementary file 1 [file final-supplementary.tex]

\documentclass{article}
\usepackage[final]{corl_2022}

\usepackage{epsfig} % for postscript graphics files
\usepackage{mathptmx} % assumes new font selection scheme installed
\usepackage{amsmath} % assumes amsmath package installed
\usepackage{amssymb}  % assumes amsmath package installed
\usepackage{tabularx}
\usepackage{multirow}
\usepackage{color}
\usepackage{url}
\usepackage{subcaption}
\usepackage{breqn}
\newcommand{\junk}[1]{}
\usepackage{algorithm2e}
\usepackage{dblfloatfix} 
\usepackage[export]{adjustbox}
\usepackage{tabulary,booktabs}
\usepackage[inkscapearea=page]{svg}
\usepackage{adjustbox}
\usepackage[legalpaper, margin=1in]{geometry}

\title{\LARGE \bf
One-Shot Transfer of Affordance Regions? AffCorrs! \\
Supplementary Meterials
%One-Shot Transfer of Semantic Region Correspondence? AffCorrs!
}

\author{
    Denis Hadjivelichkov
    \thanks{Corresponding authors are  \texttt{\{dennis.hadjivelichkov, dimitrios.kanoulas\}@ucl.ac.uk}}
    \\
  Centre for Artificial Intelligence\\
  University College London\\
  %\texttt{dennis.hadjivelichkov@ucl.ac.uk} \\
  \And
    Sicelukwanda Zwane\\
  Centre for Artificial Intelligence\\
  University College London\\
  %\texttt{sicelukwanda.zwane@ucl.ac.uk} \\
  \And
    Marc Deisenroth\\
  Centre for Artificial Intelligence\\
  University College London\\
  %\texttt{marc.deisenroth@ucl.ac.uk}
  \And
    Lourdes Agapito\\
  Department of Computer Science\\
  University College London\\
  %\texttt{lourdes.agapito@ucl.ac.uk}
  \And
    Dimitrios Kanoulas\\
  Department of Computer Science\\
  University College London\\
  %\texttt{dimitrios.kanoulas@ucl.ac.uk}
}%

\begin{document}

\maketitle

%===============================================================================

%===============================================================================

%\tableofcontents
\input{99_appendix.tex}

\bibliography{references}
\end{document}
